# Supplementary material for: MPC without Terminal Ingredients Tailored to the SEIR Compartmental Epidemic Model
Source: arXiv:2403.09151 source file (2024-06-10)
Supplement: Supplementary file 1 [file ex_supplement.tex]

% SIAM Supplemental File Template
\documentclass[review,supplement,hidelinks,onefignum,onetabnum]{siamart220329}

% SIAM Shared Information Template
% This is information that is shared between the main document and any
% supplement. If no supplement is required, then this information can
% be included directly in the main document.

% Packages and macros go here
\usepackage{amsmath} % assumes amsmath package installed
\usepackage{amssymb}  % assumes amsmath package installed
\usepackage{color}
\usepackage{graphicx}
\usepackage{booktabs}
\usepackage{color}
\usepackage{braket} % allow for \Set{...}
\usepackage{algorithm}
\usepackage{cases}
\usepackage{array}

\ifpdf
  \DeclareGraphicsExtensions{.eps,.pdf,.png,.jpg}
\else
  \DeclareGraphicsExtensions{.eps}
\fi

% Add a serial/Oxford comma by default.

% Used for creating new theorem and remark environments
\newsiamremark{remark}{Remark}
\newsiamremark{hypothesis}{Hypothesis}
\crefname{hypothesis}{Hypothesis}{Hypotheses}
\newsiamthm{claim}{Claim}
\newsiamthm{problemstatement}{Problem Statement}

% Sets running headers as well as PDF title and authors
\headers{MPC without Terminal Ingredients Tailored to SEIR Model}{W. Esterhuizen, P. Sauerteig, K. Worthmann, and S. Streif}

% Title. If the supplement option is on, then "Supplementary Material"
% is automatically inserted before the title.
\title{MPC without Terminal Ingredients Tailored to the SEIR Compartmental Epidemic Model\thanks{Submitted to the editors DATE.
\funding{This work was funded by the Fog Research Institute under contract no.~FRI-454.}}}

% Authors: full names plus addresses.
\author{Willem Esterhuizen\thanks{Imagination Corp., Chicago, IL 
  (\email{ddoe@imag.com}, \url{http://www.imag.com/\string~ddoe/}).}
\and Philipp Sauerteig\thanks{Department of Applied Mathematics, Fictional University, Boise, ID 
  (\email{ptfrank@fictional.edu}, \email{jesmith@fictional.edu}).}
\and Stefan Streif\thanks{Department of Applied Mathematics, Fictional University, Boise, ID 
	(\email{ptfrank@fictional.edu}, \email{jesmith@fictional.edu}).}
\and Karl Worthmann\thanks{Department of Applied Mathematics, Fictional University, Boise, ID 
	(\email{ptfrank@fictional.edu}, \email{jesmith@fictional.edu}).}
}
\usepackage{amsopn}

%%% Local Variables: 
%%% mode:latex
%%% TeX-master: "ex_article"
%%% End: 

\externaldocument[][nocite]{ex_article}

% Optional PDF information
\ifpdf
\hypersetup{
  pdftitle={Supplementary Materials: An Example Article},
  pdfauthor={D. Doe, P. T. Frank, and J. E. Smith}
}
\fi

\begin{document}

\maketitle

\section{A detailed example}

Here we include some equations and theorem-like environments to show
how these are labeled in a supplement and can be referenced from the
main text.
Consider the following equation:
\begin{equation}
  \label{eq:suppa}
  a^2 + b^2 = c^2.
\end{equation}
You can also reference equations such as \cref{eq:matrices,eq:bb} 
from the main article in this supplement.

\lipsum[100-101]

\begin{theorem}
An example theorem.
\end{theorem}

\lipsum[102]
 
\begin{lemma}
An example lemma.
\end{lemma}

\lipsum[103-105]

Here is an example citation: \cite{KoMa14}.

\section[Proof of Thm]{Proof of \cref{thm:bigthm}}
\label{sec:proof}

\lipsum[106-112]

\section{Additional experimental results}
\Cref{tab:smfoo} shows additional
supporting evidence. 

\begin{table}[htbp]
\footnotesize
  \caption{Example table.}\label{tab:smfoo}
\begin{center}
  \begin{tabular}{|c|c|c|} \hline
   Species & \bf Mean & \bf Std.~Dev. \\ \hline
    1 & 3.4 & 1.2 \\
    2 & 5.4 & 0.6 \\ \hline
  \end{tabular}
\end{center}
\end{table}

\bibliographystyle{siamplain}
\bibliography{references}

\end{document}
